# Supplementary material for: Frustrated pentagonal Cairo lattice in the non-collinear antiferromagnet Bi4Fe5O13F
Source: arXiv:1210.2822 source file (2012-10-10)
Supplement: Supplementary file 1 [file BiFeOF_Supplemental_Material.pdf]

# Supplemental Material

# Frustrated pentagonal Cairo lattice

# in the non-collinear antiferromagnet $Bi_4Fe_5O_{13}F$

Artem M. Abakumov[1], Dmitry Batuk[1], Alexander A. Tsirlin[2,3], Clemens Prescher[4], Leonid Dubrovinsky[4], Denis V. Sheptyakov,[5] Walter Schnelle,[2] Joke Hadermann[1], Gustaaf Van Tendeloo[1]

[1] *EMAT, University of Antwerp, Groenenborgerlaan 171, 2020 Antwerp, Belgium*

[2] *Max Planck Institute for Chemical Physics of Solids, Nöthnitzer Str. 40, 01187 Dresden, Germany*

[3]*National Institute of Chemical Physics and Biophysics, 12618 Tallinn, Estonia*

[4] *Bayerisches Geoinstitut, Universität Bayreuth, 95440 Bayreuth, Germany*

[5] *Laboratory for Neutron Scattering, Paul Scherrer Institut, CH-5232 Villigen, Switzerland*

**Details on the $Bi_4Fe_5O_{13}F$ structure analysis.**

The refinement of atomic displacement parameters (ADPs) at room temperature showed that the F1 fluorine anion and the O1 anion at the 4*a* (0,0,0) position feature ADPs 4-5 times larger than those for other atomic positions. Monitoring the behavior of ADPs for these positions with temperature and the refinement of the occupancy factors indicate that the anomalous ADPs can be attributed to the temperature-dependent random displacements away from the special positions, rather than to anion deficiency. In the room-temperature structure, we tried to place F1 and O1 into the 16*i* (*x*,0,*z*) and 8*e* (0,0,*z*) positions, respectively. The thermally-induced character of this disorder is seen from the nearly vanishing displacements at T = 1.5K: the O1 anion retains its ideal 4*a* (0,0,0) positions, whereas for the F1 anions the *x* displacement component vanishes

completely, and only a small *z* component remains. However, the presence of atomic displacements may indicate the too high crystal symmetry. Thus, the refinement in the acentric space group $P4_2bc$ was also performed. However, it did not eliminate the disorder and did not improve the reliability factors.

In the final refinements from the NPD data, the ADPs were treated in an isotropic approximation independently for every atomic position at all temperatures, except at T = 1.5K, where they there fixed to U = 0.001Å$^2$. For the SXPD data, common ADPs were refined for the Fe positions and for the anion positions. The crystal structures refined from both datasets are virtually identical. No changes, which could be attributed to structural phase transitions, have been observed in the entire temperature range of 1.5 - 700K.

The BVS calculation provides a possible reason for the displacement of the F1 anions away of the high symmetry 4*b* (0,0,1/4) position. If the F1 anions were located at 4*b* with four equivalent Bi-F bonds of 2.564Å, the BVS for the F1 anion would be 0.85(2), i.e., lower than the expected value of 1.0. The shift of the F1 anion results in one short Bi–F distance (2.35Å), two medium distances (~2.58Å) and one long distance (2.79Å). It also increases the effective valence of the F1 anions.

The disorder at the O1 position is probably linked to a slight elongation of the Fe2 - O1 bond, which is required to eliminate geometric mismatch between the linkages of the octahedral chains through the tetrahedral $Fe_2O_7$ groups and bonding between the oxygen atoms of the octahedral chains and the Bi atoms of the $Bi_4F$ groups situated between the chains.

The rutile-like chains are significantly twisted: in contrast to the parent rutile structure, the $FeO_6$ octahedra do not form an ideal eclipsed configuration along the chain (Fig. 4c). Pairs of the Fe1$O_6$ octahedra are rotated alternatively clockwise and counter-clockwise by ~ 14$^o$ around the *c* axis at the cost of a significant deformation of the Fe3$O_6$ octahedra (Fig. 4e). As a result of this twist, two trans-positioned edges of the Fe3$O_6$ octahedra form an angle of ~ 27$^o$.

**Table S1.** Selected parameters of the Rietveld refinements of the $Bi_4Fe_5O_{13}F$ structure from SXPD data.

| | | | |
|---|---|---|---|
| Formula | | $Bi_4Fe_5O_{13}F$ | |
| Space group | | $P4_2/mbc$ | |
| T, K | 10 | 298 | 673 |
| *a*, Å | 8.28460(2) | 8.29753(2) | 8.32332(3) |
| *c*, Å | 18.05373(4) | 18.06461(5) | 18.12613(8) |
| Z | | 4 | |
| Cell volume, $Å^3$ | 1239.111(4) | 1243.729(6) | 1255.735(9) |
| Calculated density, $g/cm^3$ | 7.192 | 7.165 | 7.097 |
| Radiation | | Synchrotron X-ray, λ = 0.40006 Å | |
| Parameters refined | | 20 | |
| $R_F$ , $R_P$, $R_{wP}$ | 0.015, 0.048, 0.062 | 0.021, 0.053 0.070 | 0.032, 0.076, 0.100 |

**Table S2.** Atomic parameters of $Bi_4Fe_5O_{13}F$ at 10 K, 298 K and 673 K as refined from SXPD data.

| T, K | 10 | 298 | 673 |
|---|---|---|---|
| Bi1, 16*i*, *x*,*y*,*z* | | | |
| *x* | 0.67034(4) | 0.67066(5) | 0.67158(9) |
| *y* | 0.65951(3) | 0.65961(5) | 0.65975(8) |
| *z* | 0.15703(1) | 0.15706(2) | 0.15706(3) |
| Fe1, 8*f*, 1/2,0,*z* | | | |
| *z* | 0.07945(7) | 0.07940(9) | 0.0792(1) |
| Fe2, 8*h*, *x*,*y*,0 | | | |
| *x* | 0.8504(2) | 0.8502(3) | 0.8507(5) |
| *y* | 0.8395(2) | 0.8400(3) | 0.8412(5) |
| Fe3, 4*d*, 1/2,0,1/4 | | | |
| O1, 4*a*, 0,0,0 | | | |
| O2, 16*i*, *x*,*y*,*z* | | | |
| *x* | 0.2918(5) | 0.2921(6) | 0.291(1) |
| *y* | 0.8726(6) | 0.8744(7) | 0.874(1) |
| *z* | 0.5830(3) | 0.5836(3) | 0.5822(5) |
| O3, 8*h*, *x*,*y*,0 | | | |
| *x* | 0.1399(8) | 0.140(1) | 0.139(2) |
| *y* | 0.5917(9) | 0.590(1) | 0.590(2) |
| O4, 8*g*, *x*,*x*+1/2,3/4 | | | |
| *x* | 0.3280(6) | 0.3276(7) | 0.328(1) |
| O5, 16*i*, *x*,*y*,*z* | | | |
| *x* | 0.5838(5) | 0.5823(7) | 0.583(1) |
| *y* | 0.8619(5) | 0.8598(7) | 0.860(1) |
| *z* | 0.3352(3) | 0.3353(3) | 0.3344(5) |
| F1 | 8*e**, 0,0,*z* | 16*i***, *x*,0,*z* | 16*i***, *x*,0,*z* |
| | *z* = 0.2583(7) | *x* = 0.028(2) | *x* = 0.037(3) |
| | | *z* = 0.257(1) | *z* = 0.260(2) |
| $U_{iso}$(Bi1), Å$^2$ | 0.00128(4) | 0.00652(6) | 0.0150(1) |
| $U_{iso}$(Fe1-Fe3), Å$^2$ | 0.0008(1) | 0.0047(2) | 0.0116(4) |
| $U_{iso}$(O1-O5, F1), Å$^2$ | 0.0030(6) | 0.0077(8) | 0.014(1) |

* g(F1) = 1/2;   ** g(F1) = 1/4

**Table S3.** Selected interatomic distances for $Bi_4Fe_5O_{13}F$ at 10 K, 298 K and 673 K as refined from SXPD data.

| T, K | 10 | 298 | 673 |
|---|---|---|---|
| Bi1 – O2 | 2.181(5) | 2.186(6) | 2.202(9) |
| Bi1 – O4 | 2.129(3) | 2.128(4) | 2.130(6) |
| Bi1 – O5 | 2.148(4) | 2.161(6) | 2.160(9) |
| Bi1 – O5 | 2.570(4) | 2.552(6) | 2.564(9) |
| Bi1 – F1 | 2.465(8) | 2.37(2) | 2.32(2) |
| Bi1 – F1 | 2.660(9) | 2.53(2) | 2.55(3) |
| Bi1 – F1 | | 2.61(2) | 2.64(2) |
| Bi1 – F1 | | 2.78(2) | 2.87(3) |
| | | BVS = 3.04(3) | |
| Fe1 – O2 × 2 | 2.023(4) | 2.017(5) | 2.032(9) |
| Fe1 – O3 × 2 | 1.994(5) | 1.992(6) | 1.993(10) |
| Fe1 – O5 × 2 | 2.041(5) | 2.048(6) | 2.072(9) |
| | | BVS = 2.98(2) | |
| Fe2 – O1 | 1.817(2) | 1.819(3) | 1.814(4) |
| Fe2 – O2 × 2 | 1.861(5) | 1.877(6) | 1.863(9) |
| Fe2 – O3 | 1.835(7) | 1.837(9) | 1.849(15) |
| | | BVS = 3.12(3) | |
| Fe3 – O4 × 2 | 2.016(5) | 2.022(6) | 2.029(9) |
| Fe3 – O5 × 4 | 2.039(4) | 2.049(6) | 2.045(9) |
| | | BVS = 2.81(2) | |

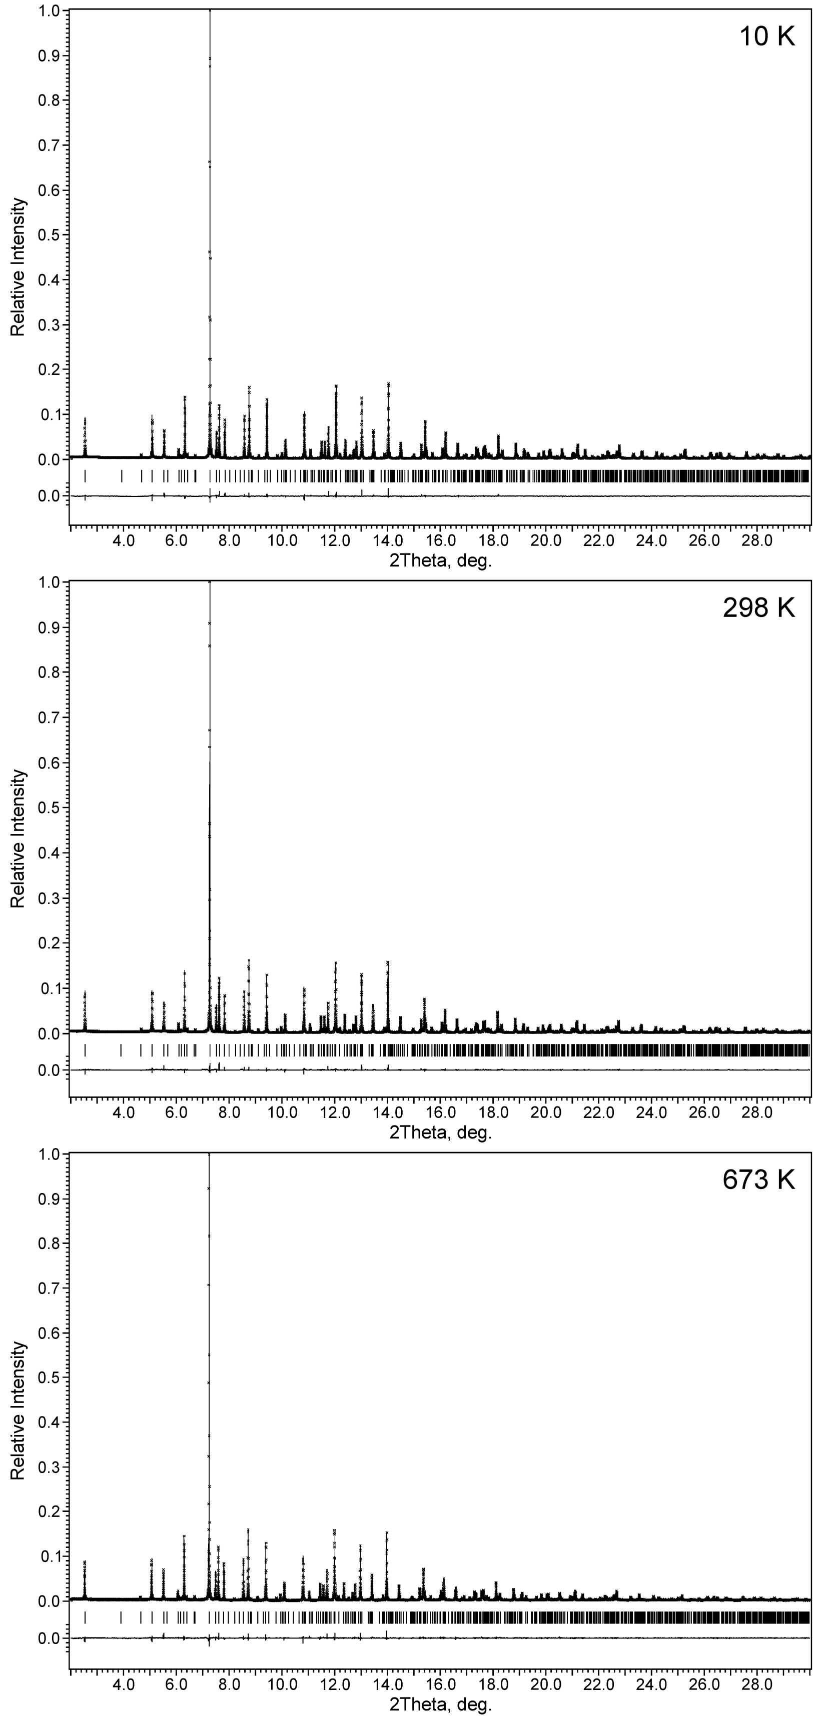


**Figure S1.** Experimental, calculated and difference SXPD profiles after Rietveld refinement of the $Bi_4Fe_5O_{13}F$ structure at 10 K, 298 K and 673 K.

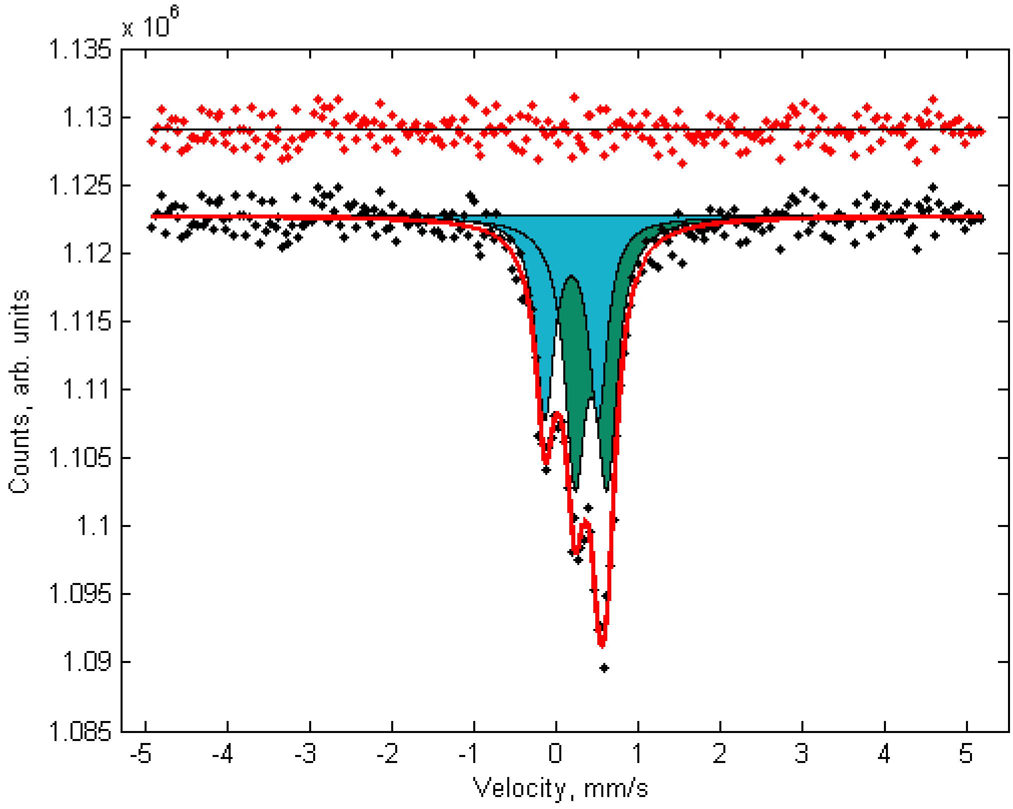


**Figure S2.** Room temperature Mössbauer spectrum for $Bi_4Fe_5O_{13}F$ and its decomposition into two doublets corresponding to the tetrahedrally (cyan) and octahedrally (green) coordinated iron.

**Table S4.** Symmetry operators of the $P_C4_2/n$ magnetic space group (86.73 in Belov-Neronova-Smirnova notations, origin shift 0,0,1/4).

| Seitz symbol | Symmetry operator | Seitz symbol | Symmetry operator |
|---|---|---|---|
| $(1\mid 0,0,0)$ | *x*, *y*, *z*, *m* | $(1\mid \frac{1}{2},\frac{1}{2},0)'$ | *x*+1/2, *y*+1/2, *z*, -*m* |
| $(2_z\mid 0,0,0)$ | -*x*, -*y*, *z*, *m* | $(2_z\mid \frac{1}{2},\frac{1}{2},0)'$ | -*x*+1/2, -*y*+1/2, *z*, -*m* |
| $(4_z\mid \frac{1}{2},\frac{1}{2},\frac{1}{2})$ | -*y*+1/2, *x*+1/2, *z*+1/2, *m* | $(4_z\mid 0,0,\frac{1}{2})'$ | -*y*, *x*, *z*+1/2, -*m* |
| $(4_z^{-1}\mid \frac{1}{2},\frac{1}{2},\frac{1}{2})$ | *y*+1/2, -*x*+1/2, *z*+1/2, *m* | $(4_z^{-1}\mid 0,0,\frac{1}{2})'$ | *y*, -*x*, *z*+1/2, -*m* |
| $(\bar{1}\mid \frac{1}{2},\frac{1}{2},0)$ | -*x*+1/2, -*y*+1/2, -*z*, *m* | $(\bar{1}\mid 0,0,0)'$ | -*x*, -*y*, -*z*, -*m* |
| $(m_z\mid \frac{1}{2},\frac{1}{2},0)$ | *x*+1/2, *y*+1/2, -*z*, *m* | $(m_z\mid 0,0,0)'$ | *x*, *y*, -*z*, -*m* |
| $(\bar{4}_z^{-1}\mid 0,0,\frac{1}{2})$ | *y*, -*x*, -*z*+1/2, *m* | $(\bar{4}_z^{-1}\mid \frac{1}{2},\frac{1}{2},\frac{1}{2})'$ | *y*+1/2, -*x*+1/2, -*z*+1/2, -*m* |
| $(\bar{4}_z\mid 0,0,\frac{1}{2})$ | -*y*, *x*, -*z*+1/2, *m* | $(\bar{4}_z\mid \frac{1}{2},\frac{1}{2},\frac{1}{2})'$ | -*y*+1/2, *x*+1/2, -*z*+1/2, -*m* |
